# Supplementary material for: Logical Consistency of Large Language Models in Fact-checking
Source: arXiv:2412.16100 source file (2025-02-28)
Supplement: Supplementary file 1 [file appendix_experimental_results_old.tex]

\section{Experiments Extended}

\begin{table*}
	\centering
	\caption{Accuracy and logical consistency on atomic queries ($1c$) before fine-tuning. }
	\begin{tabular}{llll}
		\toprule
		Model & Performance & With Context & Without Context \\
		\midrule
		Llama2 7B & Base Query Accuracy & $ 0.98 \pm 0.13 $ & $ 0.99 \pm 0.09 $ \\
		Llama2 7B & Negation Query Accuracy & $ 0.39 \pm 0.49 $ & $ 0.03 \pm 0.16 $ \\
		Llama2 7B & Consistency (when base incorrect) & $ 0.35 \pm 0.48 $ & $ 0.55 \pm 0.50 $ \\
		Llama2 7B & Consistency (when base correct) & $ 0.38 \pm 0.49 $ & $ 0.02 \pm 0.15 $ \\
		\bottomrule
	\end{tabular}
	\vspace{1em}
	
	\caption{Accuracy in different checkpoints of finetuning. Using $5000$ training samples.}
	
	\begin{tabular}{lrlll}
		\toprule
		Model & Context & Checkpoint & Base Query & Negation Query \\
		\midrule
		Llama2 7B & False & 1667 & $ 0.78 \pm 0.41 $ & $ 0.46 \pm 0.50 $ \\
		Llama2 7B & False & 3334 & $ 0.97 \pm 0.18 $ & $ 0.33 \pm 0.47 $ \\
		Llama2 7B & False & 5001 & $ 0.89 \pm 0.32 $ & $ 0.60 \pm 0.49 $ \\
		Llama2 7B & False & 6668 & $ 0.70 \pm 0.46 $ & $ 0.84 \pm 0.36 $ \\
		Llama2 7B & False & 8335 & $ 0.70 \pm 0.46 $ & $ 0.86 \pm 0.34 $ \\
		Llama2 7B & False & 10002 & $ 0.63 \pm 0.48 $ & $ 0.86 \pm 0.34 $ \\
		Llama2 7B & True & 1667 & $ 1.00 \pm 0.06 $ & $ 0.91 \pm 0.29 $ \\
		Llama2 7B & True & 3334 & $ 1.00 \pm 0.03 $ & $ 0.91 \pm 0.29 $ \\
		Llama2 7B & True & 5001 & $ 1.00 \pm 0.06 $ & $ 0.96 \pm 0.21 $ \\
		Llama2 7B & True & 6668 & $ 0.99 \pm 0.07 $ & $ 0.97 \pm 0.16 $ \\
		Llama2 7B & True & 8335 & $ 0.99 \pm 0.09 $ & $ 0.98 \pm 0.15 $ \\
		Llama2 7B & True & 10002 & $ 0.99 \pm 0.07 $ & $ 0.96 \pm 0.20 $ \\
		\bottomrule
	\end{tabular}
	\vspace{1em}
	
	\caption{Logical consistency in different checkpoints of finetuning.}
	
	
	\begin{tabular}{lrlrl}
		\toprule
		Model & Context & Checkpoint & Base Query is Correct & Logical Consistency \\
		\midrule
		Llama2 7B & False & 1667 & False & $ 0.49 \pm 0.50 $ \\
		Llama2 7B & False & 1667 & True & $ 0.45 \pm 0.50 $ \\
		Llama2 7B & False & 3334 & False & $ 0.56 \pm 0.50 $ \\
		Llama2 7B & False & 3334 & True & $ 0.33 \pm 0.47 $ \\
		Llama2 7B & False & 5001 & False & $ 0.23 \pm 0.42 $ \\
		Llama2 7B & False & 5001 & True & $ 0.58 \pm 0.49 $ \\
		Llama2 7B & False & 6668 & False & $ 0.08 \pm 0.27 $ \\
		Llama2 7B & False & 6668 & True & $ 0.81 \pm 0.39 $ \\
		Llama2 7B & False & 8335 & False & $ 0.07 \pm 0.26 $ \\
		Llama2 7B & False & 8335 & True & $ 0.84 \pm 0.37 $ \\
		Llama2 7B & False & 10002 & False & $ 0.07 \pm 0.26 $ \\
		Llama2 7B & False & 10002 & True & $ 0.83 \pm 0.38 $ \\
		Llama2 7B & True & 1667 & False & $ 0.15 \pm 0.37 $ \\
		Llama2 7B & True & 1667 & True & $ 0.91 \pm 0.28 $ \\
		Llama2 7B & True & 3334 & False & $ 0.00 \pm 0.00 $ \\
		Llama2 7B & True & 3334 & True & $ 0.91 \pm 0.29 $ \\
		Llama2 7B & True & 5001 & False & $ 0.00 \pm 0.00 $ \\
		Llama2 7B & True & 5001 & True & $ 0.96 \pm 0.21 $ \\
		Llama2 7B & True & 6668 & False & $ 0.00 \pm 0.00 $ \\
		Llama2 7B & True & 6668 & True & $ 0.97 \pm 0.16 $ \\
		Llama2 7B & True & 8335 & False & $ 0.00 \pm 0.00 $ \\
		Llama2 7B & True & 8335 & True & $ 0.98 \pm 0.15 $ \\
		Llama2 7B & True & 10002 & False & $ 0.04 \pm 0.19 $ \\
		Llama2 7B & True & 10002 & True & $ 0.96 \pm 0.20 $ \\
		\bottomrule
	\end{tabular}
	
\end{table*}


\begin{table*}
	\centering
	\caption{Average time (in seconds) required in different stages of response generation by an LLM for atomic query ($1c$). \bghosh{Do not add subgraph creation without context. Average number of triplets in the subgraph. Flipped entity time can be removed. Total time. What percentage of the entire subgraph is pruned in context creation from the subgraph. Debug the difference in LLM response time for base and negation query.}}
	\begin{tabular}{lrlllll}
		\toprule
		Model & \shortstack{Apply\\Context} & \shortstack{Subgraph\\Creation} & \shortstack{Flipped Entity\\Base Query} & \shortstack{Context\\Creation} & \shortstack{Base Query\\Response} & \shortstack{Negation Query\\Response} \\
		\midrule
		Llama2 7B & False & $ 3.08 \pm 1.73 $ & $ 0.05 \pm 0.08 $ & \textemdash & $ 0.17 \pm 0.31 $ & $ 0.24 \pm 0.39 $ \\
		Llama2 7B & True & $ 3.08 \pm 1.73 $ & $ 0.05 \pm 0.08 $ & $ 0.16 \pm 1.91 $ & $ 1.92 \pm 1.64 $ & $ 2.22 \pm 1.50 $ \\
		\bottomrule
	\end{tabular}
\end{table*}



\begin{table*}
	\centering
	\caption{Accuracy and logical consistency two-branch conjunctive query ($2i$) before fine-tuning. \bghosh{Show more detailed result for subqueries. Check numbers in 1st and 3rd row.} \bghosh{Subgraph creation can be more efficient in future.}}
	\begin{tabular}{lrrrrllll}
		\toprule
		Model & \shortstack{Apply\\Context} & \shortstack{Ground Truth\\Base Query} & \shortstack{Ground Truth\\Subquery 1} & \shortstack{Ground Truth\\Subquery 2} & \shortstack{Base Query\\Accuracy} & \shortstack{Subquery 1\\Accuracy} & \shortstack{Subquery 2\\Accuracy} & \shortstack{Logical\\Consistency} \\
		\midrule
		Llama2 7B & False & False & False & True & $ 0.02 \pm 0.15 $ & $ 0.02 \pm 0.15 $ & $ 0.98 \pm 0.15 $ & $ 0.97 \pm 0.18 $ \\
		Llama2 7B & False & False & True & False & $ 0.03 \pm 0.18 $ & $ 0.98 \pm 0.15 $ & $ 0.03 \pm 0.18 $ & $ 0.97 \pm 0.18 $ \\
		Llama2 7B & False & True & True & True & $ 0.98 \pm 0.14 $ & $ 0.99 \pm 0.12 $ & $ 0.98 \pm 0.13 $ & $ 0.99 \pm 0.11 $ \\
		Llama2 7B & True & False & False & True & $ 0.16 \pm 0.37 $ & $ 0.16 \pm 0.37 $ & $ 0.92 \pm 0.28 $ & $ 0.68 \pm 0.47 $ \\
		Llama2 7B & True & False & True & False & $ 0.21 \pm 0.41 $ & $ 0.93 \pm 0.26 $ & $ 0.21 \pm 0.41 $ & $ 0.70 \pm 0.46 $ \\
		Llama2 7B & True & True & True & True & $ 0.99 \pm 0.11 $ & $ 0.96 \pm 0.19 $ & $ 0.96 \pm 0.18 $ & $ 0.93 \pm 0.26 $ \\
		\bottomrule
	\end{tabular}
	\vspace{1em}
	
	\caption{2i after finetuning}
	\begin{tabular}{lrrrrrllll}
		\toprule
		Model & \shortstack{Apply\\Context} & \shortstack{GT\\Base} & \shortstack{GT\\Sub 1} & \shortstack{GT\\Sub 2} &
		checkpoint & \shortstack{Base Query\\Accuracy} & \shortstack{Subquery 1\\Accuracy} & \shortstack{Subquery 2\\Accuracy} & \shortstack{Logical\\Consistency} \\
		\midrule
		Llama2 7B & True & False & False & True & 500 & $ 0.34 \pm 0.47 $ & $ 0.34 \pm 0.47 $ & $ 0.92 \pm 0.27 $ & $ 0.69 \pm 0.46 $ \\
		Llama2 7B & True & False & False & True & 1000 & $ 0.75 \pm 0.43 $ & $ 0.75 \pm 0.43 $ & $ 0.72 \pm 0.45 $ & $ 0.75 \pm 0.43 $ \\
		Llama2 7B & True & False & False & True & 1500 & $ 0.89 \pm 0.32 $ & $ 0.89 \pm 0.32 $ & $ 0.49 \pm 0.50 $ & $ 0.87 \pm 0.34 $ \\
		Llama2 7B & True & False & False & True & 2000 & $ 0.63 \pm 0.48 $ & $ 0.63 \pm 0.48 $ & $ 0.94 \pm 0.23 $ & $ 0.78 \pm 0.42 $ \\
		Llama2 7B & True & False & False & True & 2500 & $ 0.87 \pm 0.34 $ & $ 0.87 \pm 0.34 $ & $ 0.82 \pm 0.38 $ & $ 0.88 \pm 0.33 $ \\
		Llama2 7B & True & False & False & True & 3000 & $ 0.86 \pm 0.34 $ & $ 0.86 \pm 0.34 $ & $ 0.85 \pm 0.35 $ & $ 0.89 \pm 0.31 $ \\
		Llama2 7B & True & False & False & True & 3500 & $ 0.77 \pm 0.42 $ & $ 0.77 \pm 0.42 $ & $ 0.87 \pm 0.34 $ & $ 0.86 \pm 0.35 $ \\
		Llama2 7B & True & False & False & True & 4000 & $ 0.73 \pm 0.44 $ & $ 0.73 \pm 0.44 $ & $ 0.96 \pm 0.20 $ & $ 0.88 \pm 0.33 $ \\
		Llama2 7B & True & False & False & True & 4500 & $ 0.83 \pm 0.38 $ & $ 0.83 \pm 0.38 $ & $ 0.88 \pm 0.33 $ & $ 0.90 \pm 0.30 $ \\
		Llama2 7B & True & False & False & True & 5000 & $ 0.74 \pm 0.44 $ & $ 0.74 \pm 0.44 $ & $ 0.94 \pm 0.23 $ & $ 0.88 \pm 0.33 $ \\
		Llama2 7B & True & False & True & False & 500 & $ 0.30 \pm 0.46 $ & $ 0.92 \pm 0.26 $ & $ 0.30 \pm 0.46 $ & $ 0.69 \pm 0.46 $ \\
		Llama2 7B & True & False & True & False & 1000 & $ 0.74 \pm 0.44 $ & $ 0.69 \pm 0.46 $ & $ 0.74 \pm 0.44 $ & $ 0.75 \pm 0.44 $ \\
		Llama2 7B & True & False & True & False & 1500 & $ 0.90 \pm 0.30 $ & $ 0.50 \pm 0.50 $ & $ 0.90 \pm 0.30 $ & $ 0.88 \pm 0.33 $ \\
		Llama2 7B & True & False & True & False & 2000 & $ 0.71 \pm 0.45 $ & $ 0.95 \pm 0.23 $ & $ 0.71 \pm 0.45 $ & $ 0.75 \pm 0.44 $ \\
		Llama2 7B & True & False & True & False & 2500 & $ 0.90 \pm 0.30 $ & $ 0.82 \pm 0.39 $ & $ 0.90 \pm 0.30 $ & $ 0.87 \pm 0.34 $ \\
		Llama2 7B & True & False & True & False & 3000 & $ 0.89 \pm 0.31 $ & $ 0.85 \pm 0.35 $ & $ 0.89 \pm 0.31 $ & $ 0.87 \pm 0.34 $ \\
		Llama2 7B & True & False & True & False & 3500 & $ 0.81 \pm 0.39 $ & $ 0.86 \pm 0.35 $ & $ 0.81 \pm 0.39 $ & $ 0.85 \pm 0.36 $ \\
		Llama2 7B & True & False & True & False & 4000 & $ 0.77 \pm 0.42 $ & $ 0.96 \pm 0.19 $ & $ 0.77 \pm 0.42 $ & $ 0.82 \pm 0.38 $ \\
		Llama2 7B & True & False & True & False & 4500 & $ 0.87 \pm 0.34 $ & $ 0.86 \pm 0.35 $ & $ 0.87 \pm 0.34 $ & $ 0.88 \pm 0.33 $ \\
		Llama2 7B & True & False & True & False & 5000 & $ 0.80 \pm 0.40 $ & $ 0.95 \pm 0.21 $ & $ 0.80 \pm 0.40 $ & $ 0.84 \pm 0.36 $ \\
		Llama2 7B & True & True & True & True & 500 & $ 0.88 \pm 0.32 $ & $ 0.96 \pm 0.21 $ & $ 0.95 \pm 0.21 $ & $ 0.82 \pm 0.38 $ \\
		Llama2 7B & True & True & True & True & 1000 & $ 0.75 \pm 0.43 $ & $ 0.82 \pm 0.39 $ & $ 0.82 \pm 0.38 $ & $ 0.68 \pm 0.46 $ \\
		Llama2 7B & True & True & True & True & 1500 & $ 0.64 \pm 0.48 $ & $ 0.68 \pm 0.47 $ & $ 0.68 \pm 0.47 $ & $ 0.59 \pm 0.49 $ \\
		Llama2 7B & True & True & True & True & 2000 & $ 0.94 \pm 0.23 $ & $ 0.98 \pm 0.15 $ & $ 0.98 \pm 0.14 $ & $ 0.92 \pm 0.26 $ \\
		Llama2 7B & True & True & True & True & 2500 & $ 0.83 \pm 0.37 $ & $ 0.93 \pm 0.26 $ & $ 0.93 \pm 0.26 $ & $ 0.84 \pm 0.37 $ \\
		Llama2 7B & True & True & True & True & 3000 & $ 0.86 \pm 0.34 $ & $ 0.94 \pm 0.24 $ & $ 0.96 \pm 0.20 $ & $ 0.87 \pm 0.34 $ \\
		Llama2 7B & True & True & True & True & 3500 & $ 0.93 \pm 0.25 $ & $ 0.95 \pm 0.22 $ & $ 0.95 \pm 0.21 $ & $ 0.90 \pm 0.30 $ \\
		Llama2 7B & True & True & True & True & 4000 & $ 0.97 \pm 0.16 $ & $ 0.99 \pm 0.11 $ & $ 0.99 \pm 0.09 $ & $ 0.97 \pm 0.16 $ \\
		Llama2 7B & True & True & True & True & 4500 & $ 0.92 \pm 0.27 $ & $ 0.95 \pm 0.22 $ & $ 0.96 \pm 0.19 $ & $ 0.90 \pm 0.29 $ \\
		Llama2 7B & True & True & True & True & 5000 & $ 0.97 \pm 0.17 $ & $ 0.98 \pm 0.14 $ & $ 0.99 \pm 0.11 $ & $ 0.96 \pm 0.20 $ \\
		\bottomrule
	\end{tabular}
	
	
	
	\vspace{1em}
	
\end{table*}
\begin{table*}
	\centering
	\caption{Average time (in seconds) required for preparing the pormpt. \bghosh{Subgraph creation time is missing.}}
	\begin{tabular}{lrllll}
		\toprule
		Model & \shortstack{Apply\\Context} & \shortstack{Context\\Creation} & \shortstack{Flipped Entity\\Base Query} & \shortstack{Flipped Entity\\Subquery 1} & \shortstack{Flipped Entity\\Subquery 2} \\
		\midrule
		Llama2 7B & False & \textemdash & $ 0.05 \pm 0.07 $ & $ 0.04 \pm 0.06 $ & $ 0.04 \pm 0.07 $ \\
		Llama2 7B & True & $ 0.12 \pm 0.18 $ & $ 0.05 \pm 0.07 $ & $ 0.04 \pm 0.06 $ & $ 0.04 \pm 0.07 $ \\
		\bottomrule
	\end{tabular}
	\vspace{1em}
	
	\caption{Average time (in seconds) required to generate LLM ressponse.}
	\begin{tabular}{lrlll}
		\toprule
		Model & \shortstack{Apply\\Context} & \shortstack{Base Query\\Response} & \shortstack{Subquery 1\\Response} & \shortstack{Subquery 2\\Response} \\
		\midrule
		Llama2 7B & False & $ 0.95 \pm 0.72 $ & $ 0.22 \pm 0.46 $ & $ 0.23 \pm 0.51 $ \\
		Llama2 7B & True & $ 1.87 \pm 1.41 $ & $ 1.49 \pm 1.54 $ & $ 1.48 \pm 1.52 $ \\
		\bottomrule
	\end{tabular}
	
\end{table*}



\begin{table*}
	\centering
	\caption{[\blue{Updated}] Accuracy and logical consistency of $2u$ queries before fine-tuning.}
	\begin{tabular}{lrrrrllll}
		\toprule
		Model & \shortstack{Apply\\Context} & \shortstack{Ground Truth\\Base Query} & \shortstack{Ground Truth\\Subquery 1} & \shortstack{Ground Truth\\Subquery 2} & \shortstack{Base Query\\Accuracy} & \shortstack{Subquery 1\\Accuracy} & \shortstack{Subquery 2\\Accuracy} & \shortstack{Logical\\Consistency} \\
		\midrule
		Llama2 7B & False & False & False & False & $ 0.02 \pm 0.12 $ & $ 0.02 \pm 0.12 $ & $ 0.02 \pm 0.12 $ & $ 0.98 \pm 0.12 $ \\
		Llama2 7B & False & True & False & True & $ 0.99 \pm 0.11 $ & $ 0.01 \pm 0.11 $ & $ 0.99 \pm 0.10 $ & $ 0.99 \pm 0.11 $ \\
		Llama2 7B & False & True & True & False & $ 0.99 \pm 0.08 $ & $ 0.99 \pm 0.09 $ & $ 0.01 \pm 0.08 $ & $ 0.99 \pm 0.08 $ \\
		Llama2 7B & False & True & True & True & $ 0.99 \pm 0.09 $ & $ 0.99 \pm 0.10 $ & $ 0.99 \pm 0.11 $ & $ 0.99 \pm 0.09 $ \\
		Llama2 7B & True & False & False & False & $ 0.57 \pm 0.50 $ & $ 0.57 \pm 0.50 $ & $ 0.57 \pm 0.50 $ & $ 0.66 \pm 0.47 $ \\
		Llama2 7B & True & True & False & True & $ 0.62 \pm 0.49 $ & $ 0.38 \pm 0.49 $ & $ 0.94 \pm 0.24 $ & $ 0.63 \pm 0.48 $ \\
		Llama2 7B & True & True & True & False & $ 0.78 \pm 0.41 $ & $ 0.95 \pm 0.22 $ & $ 0.22 \pm 0.41 $ & $ 0.77 \pm 0.42 $ \\
		Llama2 7B & True & True & True & True & $ 0.97 \pm 0.18 $ & $ 0.94 \pm 0.23 $ & $ 0.94 \pm 0.23 $ & $ 0.96 \pm 0.19 $ \\
		\bottomrule
	\end{tabular}
	\vspace{1em}
	
	
	\caption{\blue{Updated}] Accuracy and logical consistency of $2u$ after fine-tuning.}
	\begin{tabular}{lrrrrrllll}
		\toprule
		Model & \shortstack{Apply\\Context} & \shortstack{GT\\Base} & \shortstack{GT\\Sub 1} & \shortstack{GT\\Sub 2} & checkpoint & \shortstack{Base Query\\Accuracy} & \shortstack{Subquery 1\\Accuracy} & \shortstack{Subquery 2\\Accuracy} & \shortstack{Logical\\Consistency} \\
		\midrule
		Llama2 7B & True & False & False & False & 500 & $ 0.61 \pm 0.49 $ & $ 0.61 \pm 0.49 $ & $ 0.61 \pm 0.49 $ & $ 0.62 \pm 0.48 $ \\
		Llama2 7B & True & False & False & False & 1000 & $ 0.92 \pm 0.27 $ & $ 0.92 \pm 0.27 $ & $ 0.92 \pm 0.27 $ & $ 0.90 \pm 0.30 $ \\
		Llama2 7B & True & False & False & False & 1500 & $ 0.99 \pm 0.11 $ & $ 0.99 \pm 0.11 $ & $ 0.99 \pm 0.11 $ & $ 0.98 \pm 0.15 $ \\
		Llama2 7B & True & False & False & False & 2000 & $ 0.99 \pm 0.12 $ & $ 0.99 \pm 0.12 $ & $ 0.99 \pm 0.12 $ & $ 0.98 \pm 0.15 $ \\
		Llama2 7B & True & False & False & False & 2500 & $ 0.99 \pm 0.11 $ & $ 0.99 \pm 0.11 $ & $ 0.99 \pm 0.11 $ & $ 0.98 \pm 0.14 $ \\
		Llama2 7B & True & False & False & False & 3000 & $ 1.00 \pm 0.00 $ & $ 1.00 \pm 0.00 $ & $ 1.00 \pm 0.00 $ & $ 0.99 \pm 0.07 $ \\
		Llama2 7B & True & True & False & True & 500 & $ 0.76 \pm 0.42 $ & $ 0.24 \pm 0.42 $ & $ 0.98 \pm 0.12 $ & $ 0.76 \pm 0.43 $ \\
		Llama2 7B & True & True & False & True & 1000 & $ 0.96 \pm 0.19 $ & $ 0.04 \pm 0.19 $ & $ 0.97 \pm 0.18 $ & $ 0.94 \pm 0.24 $ \\
		Llama2 7B & True & True & False & True & 1500 & $ 0.83 \pm 0.37 $ & $ 0.17 \pm 0.37 $ & $ 0.98 \pm 0.14 $ & $ 0.83 \pm 0.37 $ \\
		Llama2 7B & True & True & False & True & 2000 & $ 0.95 \pm 0.21 $ & $ 0.05 \pm 0.21 $ & $ 0.99 \pm 0.09 $ & $ 0.95 \pm 0.21 $ \\
		Llama2 7B & True & True & False & True & 2500 & $ 1.00 \pm 0.07 $ & $ 0.00 \pm 0.07 $ & $ 1.00 \pm 0.06 $ & $ 0.99 \pm 0.08 $ \\
		Llama2 7B & True & True & False & True & 3000 & $ 0.90 \pm 0.30 $ & $ 0.10 \pm 0.30 $ & $ 0.98 \pm 0.13 $ & $ 0.91 \pm 0.28 $ \\
		Llama2 7B & True & True & True & False & 500 & $ 0.91 \pm 0.28 $ & $ 0.99 \pm 0.08 $ & $ 0.09 \pm 0.28 $ & $ 0.91 \pm 0.29 $ \\
		Llama2 7B & True & True & True & False & 1000 & $ 0.96 \pm 0.18 $ & $ 0.97 \pm 0.17 $ & $ 0.04 \pm 0.18 $ & $ 0.95 \pm 0.22 $ \\
		Llama2 7B & True & True & True & False & 1500 & $ 0.97 \pm 0.16 $ & $ 0.99 \pm 0.12 $ & $ 0.03 \pm 0.16 $ & $ 0.98 \pm 0.15 $ \\
		Llama2 7B & True & True & True & False & 2000 & $ 0.98 \pm 0.13 $ & $ 1.00 \pm 0.07 $ & $ 0.02 \pm 0.13 $ & $ 0.98 \pm 0.13 $ \\
		Llama2 7B & True & True & True & False & 2500 & $ 0.99 \pm 0.09 $ & $ 1.00 \pm 0.06 $ & $ 0.01 \pm 0.09 $ & $ 0.99 \pm 0.10 $ \\
		Llama2 7B & True & True & True & False & 3000 & $ 0.99 \pm 0.10 $ & $ 0.99 \pm 0.07 $ & $ 0.01 \pm 0.10 $ & $ 0.98 \pm 0.13 $ \\
		Llama2 7B & True & True & True & True & 500 & $ 0.99 \pm 0.12 $ & $ 0.99 \pm 0.11 $ & $ 0.99 \pm 0.11 $ & $ 0.99 \pm 0.12 $ \\
		Llama2 7B & True & True & True & True & 1000 & $ 1.00 \pm 0.03 $ & $ 0.97 \pm 0.18 $ & $ 0.97 \pm 0.17 $ & $ 1.00 \pm 0.03 $ \\
		Llama2 7B & True & True & True & True & 1500 & $ 1.00 \pm 0.00 $ & $ 0.99 \pm 0.12 $ & $ 0.98 \pm 0.15 $ & $ 1.00 \pm 0.00 $ \\
		Llama2 7B & True & True & True & True & 2000 & $ 1.00 \pm 0.00 $ & $ 1.00 \pm 0.06 $ & $ 0.99 \pm 0.09 $ & $ 1.00 \pm 0.00 $ \\
		Llama2 7B & True & True & True & True & 2500 & $ 1.00 \pm 0.00 $ & $ 1.00 \pm 0.06 $ & $ 1.00 \pm 0.06 $ & $ 1.00 \pm 0.00 $ \\
		Llama2 7B & True & True & True & True & 3000 & $ 1.00 \pm 0.00 $ & $ 1.00 \pm 0.05 $ & $ 0.98 \pm 0.13 $ & $ 1.00 \pm 0.00 $ \\
		
		\bottomrule
	\end{tabular}
\end{table*}






\begin{table*}
	\centering
	\caption{Combined fune-tuning on $1c$, $2i$ and $2u$ queries. Accuracy result on $1c$ test data}
	
	\begin{tabular}{lrrll}
		\toprule
		Model & Context & Checkpoint & Base Query & Negation Query \\
		\midrule
		Llama2 7B & False & 252 & $ 0.99 \pm 0.09 $ & $ 0.03 \pm 0.17 $ \\
		Llama2 7B & False & 504 & $ 0.99 \pm 0.10 $ & $ 0.04 \pm 0.19 $ \\
		Llama2 7B & False & 756 & $ 0.99 \pm 0.10 $ & $ 0.04 \pm 0.21 $ \\
		Llama2 7B & False & 1008 & $ 0.99 \pm 0.10 $ & $ 0.04 \pm 0.19 $ \\
		Llama2 7B & False & 1260 & $ 0.99 \pm 0.10 $ & $ 0.04 \pm 0.20 $ \\
		Llama2 7B & False & 1512 & $ 0.99 \pm 0.10 $ & $ 0.04 \pm 0.19 $ \\
		Llama2 7B & False & 1764 & $ 0.99 \pm 0.10 $ & $ 0.04 \pm 0.20 $ \\
		Llama2 7B & True & 252 & $ 0.86 \pm 0.35 $ & $ 0.86 \pm 0.35 $ \\
		Llama2 7B & True & 504 & $ 0.65 \pm 0.48 $ & $ 0.92 \pm 0.27 $ \\
		Llama2 7B & True & 756 & $ 0.50 \pm 0.50 $ & $ 0.95 \pm 0.22 $ \\
		Llama2 7B & True & 1008 & $ 0.49 \pm 0.50 $ & $ 0.94 \pm 0.23 $ \\
		Llama2 7B & True & 1260 & $ 0.52 \pm 0.50 $ & $ 0.94 \pm 0.24 $ \\
		Llama2 7B & True & 1512 & $ 0.52 \pm 0.50 $ & $ 0.93 \pm 0.25 $ \\
		Llama2 7B & True & 1764 & $ 0.51 \pm 0.50 $ & $ 0.94 \pm 0.24 $ \\
		\bottomrule
	\end{tabular}
	\vspace{1em}
	
	\caption{Logical consistency on $1c$ test data}
	\begin{tabular}{lrrrl}
		\toprule
		Model & Context & Base Query is Correct & Checkpoint & Logical Consistency \\
		\midrule
		Llama2 7B & False & False & 252 & $ 0.50 \pm 0.51 $ \\
		Llama2 7B & False & False & 504 & $ 0.50 \pm 0.51 $ \\
		Llama2 7B & False & False & 756 & $ 0.54 \pm 0.50 $ \\
		Llama2 7B & False & False & 1008 & $ 0.53 \pm 0.50 $ \\
		Llama2 7B & False & False & 1260 & $ 0.55 \pm 0.50 $ \\
		Llama2 7B & False & False & 1512 & $ 0.59 \pm 0.50 $ \\
		Llama2 7B & False & False & 1764 & $ 0.56 \pm 0.50 $ \\
		Llama2 7B & False & True & 252 & $ 0.03 \pm 0.16 $ \\
		Llama2 7B & False & True & 504 & $ 0.03 \pm 0.18 $ \\
		Llama2 7B & False & True & 756 & $ 0.04 \pm 0.20 $ \\
		Llama2 7B & False & True & 1008 & $ 0.04 \pm 0.18 $ \\
		Llama2 7B & False & True & 1260 & $ 0.04 \pm 0.19 $ \\
		Llama2 7B & False & True & 1512 & $ 0.03 \pm 0.18 $ \\
		Llama2 7B & False & True & 1764 & $ 0.04 \pm 0.19 $ \\
		Llama2 7B & True & False & 252 & $ 0.07 \pm 0.25 $ \\
		Llama2 7B & True & False & 504 & $ 0.05 \pm 0.21 $ \\
		Llama2 7B & True & False & 756 & $ 0.03 \pm 0.17 $ \\
		Llama2 7B & True & False & 1008 & $ 0.04 \pm 0.20 $ \\
		Llama2 7B & True & False & 1260 & $ 0.04 \pm 0.21 $ \\
		Llama2 7B & True & False & 1512 & $ 0.05 \pm 0.22 $ \\
		Llama2 7B & True & False & 1764 & $ 0.04 \pm 0.21 $ \\
		Llama2 7B & True & True & 252 & $ 0.85 \pm 0.36 $ \\
		Llama2 7B & True & True & 504 & $ 0.90 \pm 0.30 $ \\
		Llama2 7B & True & True & 756 & $ 0.93 \pm 0.26 $ \\
		Llama2 7B & True & True & 1008 & $ 0.92 \pm 0.26 $ \\
		Llama2 7B & True & True & 1260 & $ 0.92 \pm 0.27 $ \\
		Llama2 7B & True & True & 1512 & $ 0.92 \pm 0.27 $ \\
		Llama2 7B & True & True & 1764 & $ 0.92 \pm 0.27 $ \\
		\bottomrule
	\end{tabular}    
\end{table*}

\begin{table*}
	
	
	\caption{Accuracy and logical consistency on $2i$ test data.}
	\begin{tabular}{lrrrrrllll}
		\toprule
		Model & \shortstack{Apply\\Context} & \shortstack{GT\\Base} & \shortstack{GT\\Sub 1} & \shortstack{GT\\Sub 2} & checkpoint & \shortstack{Base Query\\Accuracy} & \shortstack{Subquery 1\\Accuracy} & \shortstack{Subquery 2\\Accuracy} & \shortstack{Logical\\Consistency} \\
		\midrule
		Llama2 7B & True & False & False & True & 252 & $ 0.30 \pm 0.46 $ & $ 0.30 \pm 0.46 $ & $ 0.85 \pm 0.35 $ & $ 0.65 \pm 0.48 $ \\
		Llama2 7B & True & False & False & True & 504 & $ 0.58 \pm 0.49 $ & $ 0.58 \pm 0.49 $ & $ 0.61 \pm 0.49 $ & $ 0.69 \pm 0.46 $ \\
		Llama2 7B & True & False & False & True & 756 & $ 0.73 \pm 0.45 $ & $ 0.73 \pm 0.45 $ & $ 0.45 \pm 0.50 $ & $ 0.74 \pm 0.44 $ \\
		Llama2 7B & True & False & False & True & 1008 & $ 0.71 \pm 0.45 $ & $ 0.71 \pm 0.45 $ & $ 0.45 \pm 0.50 $ & $ 0.74 \pm 0.44 $ \\
		Llama2 7B & True & False & False & True & 1260 & $ 0.69 \pm 0.46 $ & $ 0.69 \pm 0.46 $ & $ 0.46 \pm 0.50 $ & $ 0.73 \pm 0.44 $ \\
		Llama2 7B & True & False & False & True & 1512 & $ 0.70 \pm 0.46 $ & $ 0.70 \pm 0.46 $ & $ 0.45 \pm 0.50 $ & $ 0.71 \pm 0.45 $ \\
		Llama2 7B & True & False & False & True & 1764 & $ 0.68 \pm 0.47 $ & $ 0.68 \pm 0.47 $ & $ 0.48 \pm 0.50 $ & $ 0.72 \pm 0.45 $ \\
		Llama2 7B & True & False & True & False & 252 & $ 0.36 \pm 0.48 $ & $ 0.85 \pm 0.36 $ & $ 0.36 \pm 0.48 $ & $ 0.65 \pm 0.48 $ \\
		Llama2 7B & True & False & True & False & 504 & $ 0.62 \pm 0.48 $ & $ 0.61 \pm 0.49 $ & $ 0.62 \pm 0.48 $ & $ 0.69 \pm 0.46 $ \\
		Llama2 7B & True & False & True & False & 756 & $ 0.76 \pm 0.42 $ & $ 0.46 \pm 0.50 $ & $ 0.76 \pm 0.42 $ & $ 0.76 \pm 0.42 $ \\
		Llama2 7B & True & False & True & False & 1008 & $ 0.75 \pm 0.44 $ & $ 0.47 \pm 0.50 $ & $ 0.75 \pm 0.44 $ & $ 0.74 \pm 0.44 $ \\
		Llama2 7B & True & False & True & False & 1260 & $ 0.74 \pm 0.44 $ & $ 0.46 \pm 0.50 $ & $ 0.74 \pm 0.44 $ & $ 0.75 \pm 0.44 $ \\
		Llama2 7B & True & False & True & False & 1512 & $ 0.73 \pm 0.44 $ & $ 0.47 \pm 0.50 $ & $ 0.73 \pm 0.44 $ & $ 0.75 \pm 0.43 $ \\
		Llama2 7B & True & False & True & False & 1764 & $ 0.72 \pm 0.45 $ & $ 0.47 \pm 0.50 $ & $ 0.72 \pm 0.45 $ & $ 0.74 \pm 0.44 $ \\
		Llama2 7B & True & True & True & True & 252 & $ 0.93 \pm 0.25 $ & $ 0.92 \pm 0.27 $ & $ 0.92 \pm 0.27 $ & $ 0.84 \pm 0.36 $ \\
		Llama2 7B & True & True & True & True & 504 & $ 0.71 \pm 0.45 $ & $ 0.75 \pm 0.43 $ & $ 0.75 \pm 0.43 $ & $ 0.66 \pm 0.47 $ \\
		Llama2 7B & True & True & True & True & 756 & $ 0.54 \pm 0.50 $ & $ 0.59 \pm 0.49 $ & $ 0.61 \pm 0.49 $ & $ 0.61 \pm 0.49 $ \\
		Llama2 7B & True & True & True & True & 1008 & $ 0.55 \pm 0.50 $ & $ 0.60 \pm 0.49 $ & $ 0.60 \pm 0.49 $ & $ 0.62 \pm 0.49 $ \\
		Llama2 7B & True & True & True & True & 1260 & $ 0.56 \pm 0.50 $ & $ 0.62 \pm 0.48 $ & $ 0.62 \pm 0.49 $ & $ 0.61 \pm 0.49 $ \\
		Llama2 7B & True & True & True & True & 1512 & $ 0.58 \pm 0.49 $ & $ 0.62 \pm 0.49 $ & $ 0.61 \pm 0.49 $ & $ 0.63 \pm 0.48 $ \\
		Llama2 7B & True & True & True & True & 1764 & $ 0.58 \pm 0.49 $ & $ 0.62 \pm 0.49 $ & $ 0.64 \pm 0.48 $ & $ 0.61 \pm 0.49 $ \\
		\bottomrule
	\end{tabular}
	\vspace{1em}
	
	\caption{Accuracy and logical consistency on $2u$ test dataset. \red{What is the meaning of standard deviation? The performance on 2u and 2i is not good. We should try more samples. How many epochs does LORA usually need?} }
	\begin{tabular}{lrrrrrllll}
		\toprule
		Model & \shortstack{Apply\\Context} & \shortstack{GT\\Base} & \shortstack{GT\\Sub 1} & \shortstack{GT\\Sub 2} & checkpoint & \shortstack{Base Query\\Accuracy} & \shortstack{Subquery 1\\Accuracy} & \shortstack{Subquery 2\\Accuracy} & \shortstack{Logical\\Consistency} \\
		\midrule
		Llama2 7B & True & False & False & False & 252 & $ 0.69 \pm 0.46 $ & $ 0.69 \pm 0.46 $ & $ 0.69 \pm 0.46 $ & $ 0.65 \pm 0.48 $ \\
		Llama2 7B & True & False & False & False & 504 & $ 0.82 \pm 0.39 $ & $ 0.82 \pm 0.39 $ & $ 0.82 \pm 0.39 $ & $ 0.76 \pm 0.43 $ \\
		Llama2 7B & True & False & False & False & 756 & $ 0.86 \pm 0.35 $ & $ 0.86 \pm 0.35 $ & $ 0.86 \pm 0.35 $ & $ 0.80 \pm 0.40 $ \\
		Llama2 7B & True & False & False & False & 1008 & $ 0.82 \pm 0.38 $ & $ 0.82 \pm 0.38 $ & $ 0.82 \pm 0.38 $ & $ 0.78 \pm 0.42 $ \\
		Llama2 7B & True & False & False & False & 1260 & $ 0.82 \pm 0.38 $ & $ 0.82 \pm 0.38 $ & $ 0.82 \pm 0.38 $ & $ 0.77 \pm 0.42 $ \\
		Llama2 7B & True & False & False & False & 1512 & $ 0.83 \pm 0.37 $ & $ 0.83 \pm 0.37 $ & $ 0.83 \pm 0.37 $ & $ 0.77 \pm 0.42 $ \\
		Llama2 7B & True & False & False & False & 1764 & $ 0.82 \pm 0.38 $ & $ 0.82 \pm 0.38 $ & $ 0.82 \pm 0.38 $ & $ 0.78 \pm 0.42 $ \\
		Llama2 7B & True & True & False & True & 252 & $ 0.44 \pm 0.50 $ & $ 0.56 \pm 0.50 $ & $ 0.89 \pm 0.32 $ & $ 0.47 \pm 0.50 $ \\
		Llama2 7B & True & True & False & True & 504 & $ 0.26 \pm 0.44 $ & $ 0.74 \pm 0.44 $ & $ 0.70 \pm 0.46 $ & $ 0.43 \pm 0.50 $ \\
		Llama2 7B & True & True & False & True & 756 & $ 0.16 \pm 0.37 $ & $ 0.84 \pm 0.37 $ & $ 0.51 \pm 0.50 $ & $ 0.50 \pm 0.50 $ \\
		Llama2 7B & True & True & False & True & 1008 & $ 0.17 \pm 0.38 $ & $ 0.83 \pm 0.38 $ & $ 0.52 \pm 0.50 $ & $ 0.51 \pm 0.50 $ \\
		Llama2 7B & True & True & False & True & 1260 & $ 0.22 \pm 0.41 $ & $ 0.78 \pm 0.41 $ & $ 0.54 \pm 0.50 $ & $ 0.51 \pm 0.50 $ \\
		Llama2 7B & True & True & False & True & 1512 & $ 0.22 \pm 0.42 $ & $ 0.78 \pm 0.42 $ & $ 0.54 \pm 0.50 $ & $ 0.50 \pm 0.50 $ \\
		Llama2 7B & True & True & False & True & 1764 & $ 0.20 \pm 0.40 $ & $ 0.80 \pm 0.40 $ & $ 0.55 \pm 0.50 $ & $ 0.50 \pm 0.50 $ \\
		Llama2 7B & True & True & True & False & 252 & $ 0.67 \pm 0.47 $ & $ 0.89 \pm 0.31 $ & $ 0.33 \pm 0.47 $ & $ 0.66 \pm 0.47 $ \\
		Llama2 7B & True & True & True & False & 504 & $ 0.46 \pm 0.50 $ & $ 0.68 \pm 0.47 $ & $ 0.54 \pm 0.50 $ & $ 0.56 \pm 0.50 $ \\
		Llama2 7B & True & True & True & False & 756 & $ 0.36 \pm 0.48 $ & $ 0.53 \pm 0.50 $ & $ 0.64 \pm 0.48 $ & $ 0.54 \pm 0.50 $ \\
		Llama2 7B & True & True & True & False & 1008 & $ 0.39 \pm 0.49 $ & $ 0.52 \pm 0.50 $ & $ 0.61 \pm 0.49 $ & $ 0.56 \pm 0.50 $ \\
		Llama2 7B & True & True & True & False & 1260 & $ 0.43 \pm 0.50 $ & $ 0.55 \pm 0.50 $ & $ 0.57 \pm 0.50 $ & $ 0.57 \pm 0.50 $ \\
		Llama2 7B & True & True & True & False & 1512 & $ 0.41 \pm 0.49 $ & $ 0.55 \pm 0.50 $ & $ 0.59 \pm 0.49 $ & $ 0.55 \pm 0.50 $ \\
		Llama2 7B & True & True & True & False & 1764 & $ 0.41 \pm 0.49 $ & $ 0.55 \pm 0.50 $ & $ 0.59 \pm 0.49 $ & $ 0.56 \pm 0.50 $ \\
		Llama2 7B & True & True & True & True & 252 & $ 0.92 \pm 0.27 $ & $ 0.88 \pm 0.32 $ & $ 0.88 \pm 0.32 $ & $ 0.92 \pm 0.28 $ \\
		Llama2 7B & True & True & True & True & 504 & $ 0.73 \pm 0.44 $ & $ 0.70 \pm 0.46 $ & $ 0.69 \pm 0.46 $ & $ 0.72 \pm 0.45 $ \\
		Llama2 7B & True & True & True & True & 756 & $ 0.58 \pm 0.49 $ & $ 0.52 \pm 0.50 $ & $ 0.52 \pm 0.50 $ & $ 0.62 \pm 0.49 $ \\
		Llama2 7B & True & True & True & True & 1008 & $ 0.59 \pm 0.49 $ & $ 0.54 \pm 0.50 $ & $ 0.53 \pm 0.50 $ & $ 0.63 \pm 0.48 $ \\
		Llama2 7B & True & True & True & True & 1260 & $ 0.59 \pm 0.49 $ & $ 0.54 \pm 0.50 $ & $ 0.54 \pm 0.50 $ & $ 0.63 \pm 0.48 $ \\
		Llama2 7B & True & True & True & True & 1512 & $ 0.59 \pm 0.49 $ & $ 0.53 \pm 0.50 $ & $ 0.56 \pm 0.50 $ & $ 0.63 \pm 0.48 $ \\
		Llama2 7B & True & True & True & True & 1764 & $ 0.60 \pm 0.49 $ & $ 0.53 \pm 0.50 $ & $ 0.55 \pm 0.50 $ & $ 0.62 \pm 0.49 $ \\
		\bottomrule
	\end{tabular}
\end{table*}


\begin{figure}
	\centering
	\includegraphics[scale=0.5]{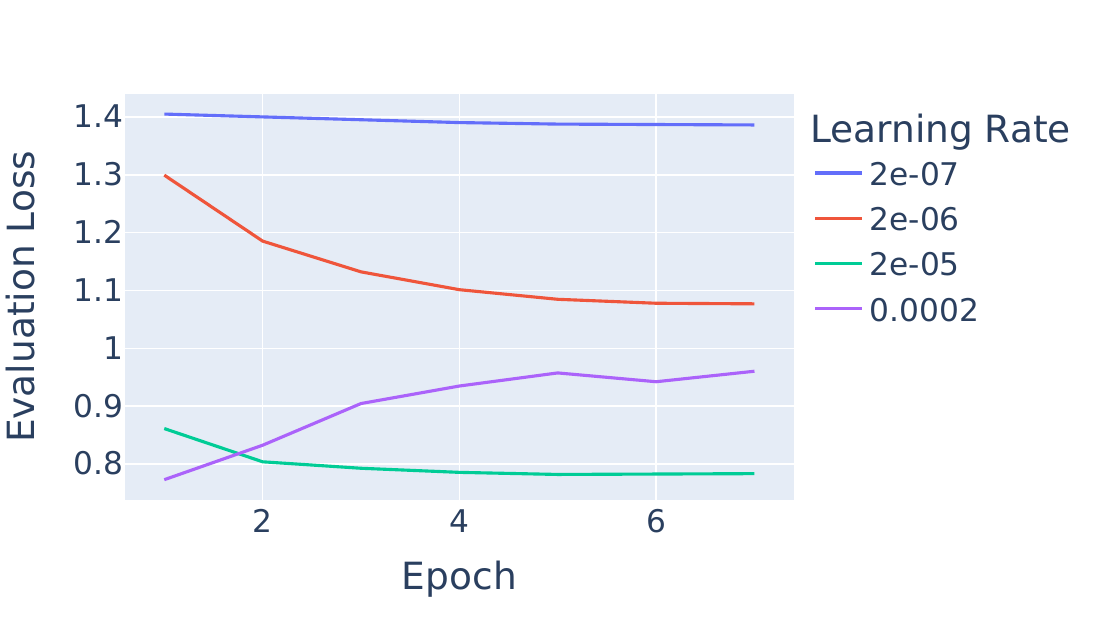}
	\includegraphics[scale=0.5]{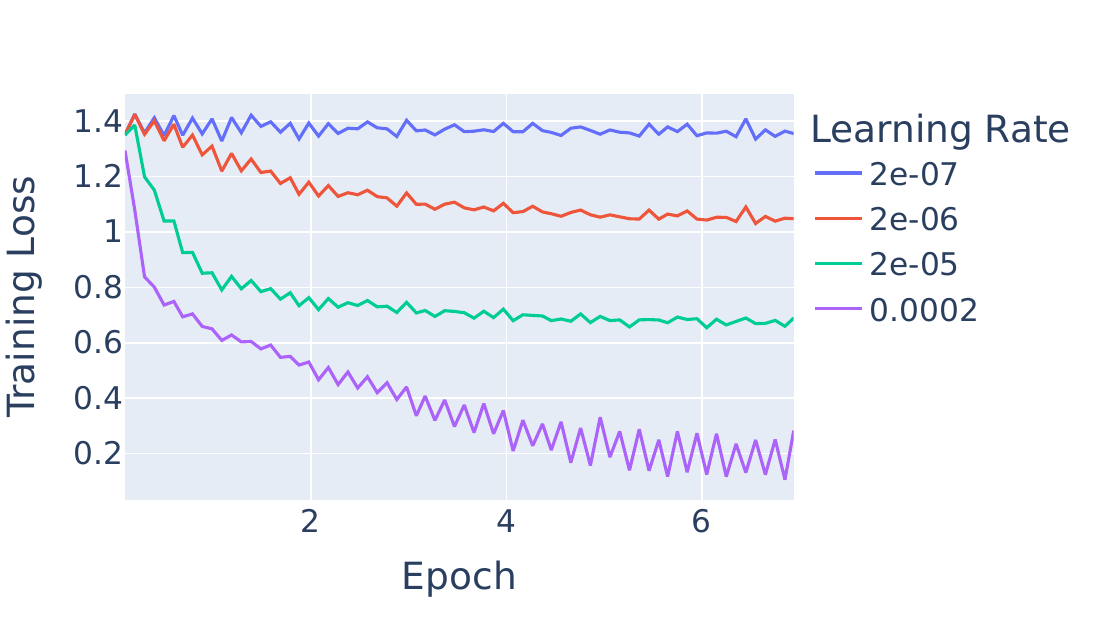}
\end{figure}
