# Supplementary material for: Logical Consistency of Large Language Models in Fact-checking
Source: arXiv:2412.16100 source file (2025-02-28)
Supplement: Supplementary file 2 [file appendix_old.tex]

\section{Preliminary}
\paragraph{Basic Notations of LLM Token Generation~\cite{liang2021towards}.}

Given some context $ c $ and a target vocabulary $ V $ consisting of a discrete set of word tokens, a language model $ p_{\theta} $ with parameters $ \theta $ aims to predict a distribution over the next candidates in $ V $ over multiple time steps until a maximum step $ T $ is reached.

\begin{align}
    p_{\theta}(w_t|c_{t-1}) = p_{\theta}(w_t|w_0, w_1, \cdots, w_{t-1}), \forall t \leq T
\end{align}

$ p_{\theta}(w_t|c_{t-1}) $ is implemented via two functions: an embedding function $ e $ over the vocabulary $ V $ (either pre-trained word embeddings or trainable embeddings), and an encoding function $ f $ over the context $ c_{t-1} $. The probability of a given next token $ w_t $ is then equivalent to a softmax over distances between the token embedding $ e(w_t) $ and context embedding $ f(c_{t-1}) $:

\begin{align}
    p_{\theta}(w_t|w_0, w_1, \cdots, w_{t-1}) = \frac{exp(e(w_t)^Tf(c_{t-1}))}{\sum_{w \in V}exp(e(w)^Tf(c_{t-1}))}
\end{align}

When using a transformer LM such as GPT-2, one can define the encoded context $ f(c_{t-1}) $ to consist of key-value pairs from the past.

\begin{align}
    f(c_{t-1}) = [(K^{(1)}_{t-1}, V^{(1)}_{t-1}), \cdots, (K^{(t)}_{t-1}, V^{(t)}_{t-1})],
\end{align}

where $ (K^{(1)}_{t-1}, V^{(1)}_{t-1}) $  corresponds to the key-value pairs from the $ i $-th transformer layer generated from time steps $ 0 $ to $ t - 1 $.



\paragraph{Fine-grained Local Biases.}

Consider the generation of word $ w_{t} $ given a context $ c^{(1)}_{t-1} $ describing the first social group. Change the context to $ c^{(2)}_{t-1} $ such that it describes the second social group. This can be done via simple word replacement for a predefined set of gender pairs.


A model's generation at time $ t $ is said to be locally biased if:

\begin{align}
    p_{\theta}(w_t|c^{(1)}_{t-1}) \ne p_{\theta}(w_t|c^{(2)}_{t-1})
\end{align}


To measure local biases across the vocabulary, simple $ f $-divergence between the probability distributions can be used.

Local biases generalizes WEAT and SEAT tests for computing biased assiciation in word and sentence embeddings.

\paragraph{High-level Global Biases.} Global biases take a more holistic view that considers the semantics of the generated sentence. 


Let $ s^{(1)} $ and $ s^{(2)} $ be the complete generated sentences for the two different contexts. 

A model's generation at time $ t $ is globally biased if 

\begin{align}
    g(s^{(1)}) \ne g(s^{(2)})
\end{align}

where $ g(\cdot) $
contains sentiment and regard measures to capture representational biases in the semantics of the entire phrases.


\section{Techniques for Measuring Bias}

\paragraph{Sentence Encoder Assiciation Test (SEAT)} SEAT is an extension of word embedding association test (WEAT) to sentence-level representations. WEAT makes use of four sets of words: two set of bias \textit{attribute} words and two sets of \textit{target} words. The attribute word sets characterize a type of bias. For example, the attribute word sets \{man, he, him, ...\} and \{woman, she, her, ...\} could be used for gender bias. The target word sets characterize particular concepts. For example, the target word sets \{faminly, child, parent, ...\} and \{work, office, profession, ...\} could be used to characterize the concepts of family and career, respectively. WEAT evaluates whether the representations for word from one particular attribute word set tend to be more closely associated with the representations for words from one particular target word set. For example, if female attribute words are more close to family, and similarly male are more closely related to careers, then this indicate bias. 
\textbf{Paper source: } \url{https://arxiv.org/pdf/2110.08527.pdf}


\paragraph{StereoSet} This is a crowd-sourced dataset for measuring \textbf{four} types of bias in language models. Each StereoSet example consists of a context sentence, for example `\textit{our housekeeper is [MASK]'} and a set of three candidate associations (completions) for that sentence\textemdash one being stereotypical, another being anti-stereotypical, and a third being unrelated. 
\begin{itemize}
    \item \textbf{Stereotypical:} \textit{Our housekeeper is Mexican}.
    \item \textbf{Anti-stereotypical:} \textit{Our housekeeper is American}.
    \item \textbf{Unrelated:} \textit{Our housekeeper is a computer}.
\end{itemize}

Bias measurement boils down to computing the percentage of examples that an LLM predicts from the stereotypical class to the anti-stereotypical class. This is called \textbf{stereotype score} of the model

This dataset also computes the \textbf{language modeling score}, which is measured as the percentage of unrelated association vs stereo or anti-stereotypical association.


\paragraph{Crowd-sourced Stereotype Pairs (CorwS-Pairs} CrowS-Pairs is a crowd-sourced dataset that consists of pairs of minimally distant sentences: sentences that differe only with respect to a small number of tokens. 
\begin{itemize}
    \item The first sentence in each pair reflects a stereotype about a historically disadvantaged group in the USA. For example, the sentence `people who live in trailers are alcoholics' reflects a possible socio-economic stereotype.
    \item  The second sentence in each pair then \textit{violates} the stereotype introduced in the first sentence. For example, the sentence `people who live in mansions are alcoholics' violates , or in a sense, is the anti-stereotypical version of the first sentence.
\end{itemize}

Bias measurement is based on the pseudo-log-likelihood of generating stereotypical sentences vs anti-stereotypical sentences.



\section{Related Work}
\paragraph{Few-shot instruction prompts for pretrained language models to detect social biases}

The goal is to use a few-shot instruction-based method for prompting pre-trained language models for detecting biased responses~\cite{prabhumoye2021few}.

\textbf{Zero shot case:} input to the model $M$ is $ p = [\textbf{`Post:'}; Q; \textbf{`Question:'}; d; \textbf{`Answer:'}]$.

\begin{itemize}
    \item Example of $ Q $ is \textit{Newbie here, saw this on twitter, I am trying as I am so tired of conservatives being blocked and banned.}

    \item $ d $ is the definition of bias. For example, \textit{Could this post be considered offensive, disrespectful, or toxic to anyone/someone?}
\end{itemize}

Then check if $ \Pr_M(\textbf{`Yes'} | p) > \Pr_M(\textbf{`No'} | p) $ 


In the few-shot case, the authors use a labeled dataset $ D $ where each sample $ (x_i, c_i) $ is a tuple of textual post and the class of the post respectively. The definition $ d $ for bias is also known apriori. The input $ p $ to the model is a concatenation of the strings: $ p = [x_1; d; c_1; \cdots; x_k; d; c_k; Q; d] $.



\subsection*{Experimental Details.}

Datasets: 

\begin{itemize}
    \item StereoSet~\cite{nadeem2020stereoset}  is a recently proposed dataset of simple contexts with human annotations for various possible next word completions that range from unbiased to biased (showing stereotypes). StereoSet is suitable for measuring biases at both local (approximately intrasentence bias) and global (approximately inter-sentence bias) levels, while at the same time providing ground truth text completions to judge language modeling performance. Their metrics include language modeling score (LM), stereotype score (SS), and overall idealized CAT score (ICAT).

    \item Simple contexts as proposed by~\cite{sheng2019woman} to test LMs with certain context templates describing gender, race, religion, and other social constructs. 

    \item Social Bias Frames (SBIC): This dataset (Sap et al., 2020) contains ﬁne-grained categorization of textual comments to better model the pragmatic frames in which people project social biases and stereotypes onto others. It contains four binary classiﬁcation tasks and one multi-class classiﬁcation task (\%age positive samples in test set are shown in brackets): (1) offensive task (57.8\% pos): predict if the text is offensive or not, (2) intent task (53.1\% pos): predict if the text is an intentional insult or not, (3) lewd task (9.6\% pos): predict if the text contains lewd language or not, (4) group task (41.1\% pos): predict if the text is offensive to a group or an individual, and (5) target group (WHO) task: if the text is offensive to a group then identify the group targeted in the text. We design the target group identiﬁcation as a seven-way classiﬁcation task where the target group categories are - body, culture, disabled, gender, race, social, victim. Sap et al. (2020) treat these ﬁve tasks as a single generative task where the entire frame is generated token by token. We treat them as ﬁve separate classiﬁcation tasks. 

    \item HASOC
\end{itemize}


\section{Graph of Thoughts}
The key idea is to analyze the reasoning of an LLM by converting LLM responses into a graph.

For multiple options QA (question answering) tasks, one idea is to convert the multi-class classification task to ensemble of binary classification tasks and see how consistent the LLM is in answering the same questions but presented differently. 

\textbf{Remark.} Most bias benchmarks to detect stereotypes and harmful responses may be biased, where human annotators put ground-truth labels. 
